# Supplementary material for: FlashST: A Simple and Universal Prompt-Tuning Framework for Traffic Prediction
Source: arXiv:2405.17898 source file (2024-05-28)
Supplement: Supplementary file 1 [file appendix.tex]

\section{Appendix}
\label{sec:appendix}
% In the appendix, we primarily provide additional details regarding the experimental setup, statistical information about the dataset, and an overview of the baseline model.
The appendix provides additional details concerning the experimental setup, statistical information about the dataset, an overview of the baseline model, \textcolor{red}{complexity analysis of the proposed method and the limitations of this work.}

% \textbf{Experimental Description.} In our model, the hidden units $d$, $d_t$ and $d_r$ are set to 32, and the number of layers in the spatial and temporal encoder is set to 2. During the pre-training phase, we conduct alternating training for 300 epochs on the four pre-training datasets, while in the prompt-tuning phase, we perform fine-tuning for 20 epochs. For the baseline and full fine-tuning setups, we set a maximum of 100 epochs for training. The batch size is set to 64 for both phase and all of the baselines.

\textbf{Experimental Description. } 
We configure the model with 32 hidden units for $d$, $d_t$, and $d_r$, while employing a spatial and temporal encoder with 2 layers. The pre-training phase involves alternating training for 300 epochs on the four pre-training datasets. Subsequently, we conduct fine-tuning for 20 epochs during the prompt-tuning phase. In both the baseline and full fine-tuning setups, the maximum number of training epochs is limited to 100. Furthermore, a batch size of 64 is employed for both phases and all baselines. \textcolor{red}{For dataset-specific parameters involved in the baseline (\eg~node embeddings), we initialize them randomly and set them as trainable during the prompt fine-tuning phase. Additionally, the final regression layers of some baseline model are set to trainable to ensure accurate numerical predictions.}

\textbf{Data Description.} 
% The pre-training dataset comprises records of traffic flow conditions in various streets and cities across California, which can be sourced from~\cite{Song2020spatial}. For the test datasets, PEMS07(M)~\cite{yu2018spatio}, CA-D5~\cite{liu2023largest}, ChengDu-DIDI~\cite{lu2022spatio}, and NYC Citi Bike~\cite{ye2021coupled} recorded different types of ST data, including traffic speed, traffic flow, traffic index, and bicycle usage. Detailed statistics of each dataset are listed in Table~\ref{tab:Dataset_pretrain} and Table~\ref{tab:Dataset_test}.
The pre-training dataset consists of records detailing traffic flow conditions across various streets and cities in California, which can be obtained from~\cite{Song2020spatial}. The test datasets, including PEMS07(M)\cite{yu2018spatio}, CA-D5\cite{liu2023largest}, ChengDu-DIDI~\cite{lu2022spatio}, and NYC Citi Bike~\cite{ye2021coupled}, provide diverse types of spatio-temporal (ST) data, encompassing traffic speed, traffic flow, traffic index, and bicycle usage. Detailed statistics for each dataset can be found in Table~\ref{tab:Dataset_pretrain} and Table~\ref{tab:Dataset_test}.

% \textbf{Baseline Model.} To facilitate discussion, we categorize existing models into four groups: spatio-temporal prediction methods based on RNNs, GNNs, attention mechanism, and ordinary differential equation.
\textbf{Baseline Models:} To facilitate effective discussions, we categorize baselines into four groups based on their approach to spatio-temporal prediction: methods utilizing RNNs, GNNs, attention mechanisms, and ordinary differential equations.

\noindent \textbf{RNN-based Spatio-Temporal Prediction Model:}
\begin{itemize}[leftmargin=*]
% \item \textbf{AGCRN}~\cite{bai2020adaptive}: This method utilizes learnable node embeddings combined with RNNs to encode personalized spatio-temporal patterns of regions.
\item \textbf{AGCRN}\cite{bai2020adaptive}: This method incorporates RNNs with learnable node embeddings to capture personalized spatio-temporal patterns of regions.
% \item \textbf{MSDR}~\cite{liu2022msdr}: The model introduces a variant of RNNs to alleviate the problem of long-term information forgetting and combines it with graph networks to capture spatio-temporal correlations.
\item \textbf{MSDR}\cite{liu2022msdr}: This model addresses the issue of long-term information forgetting in RNNs by introducing a variant of RNNs. It further combines this variant with GNNs to capture spatio-temporal correlations.
\end{itemize}

% \noindent \textbf{Spatial temporal prediction model based on GNNs:}
\textbf{GNN-based Spatio-Temporal Prediction Model:}
\begin{itemize}[leftmargin=*]
% \item \textbf{TGCN}~\cite{Zhao2020TGCN}: This model employs RNNs and GCNs to separately model temporal dependencied and spatial correlations.
\item \textbf{TGCN}\cite{Zhao2020TGCN}: This model combines RNNs and GCNs to separately model temporal dependencies and spatial correlations.
% \item \textbf{STGCN}~\cite{yu2018spatio}: This method utilizes gated convolutional networks to encode temporal dependencies and GCNs to capture local spatial relationships.
\item \textbf{STGCN}\cite{yu2018spatio}: This method utilizes gated convolutional networks to encode temporal dependencies and GCNs to capture local spatial relationships.
% \item \textbf{GWN}~\cite{wu2019graph}: This approach adopts a learnable graph structure to model spatial correlations, while TCNs are used to extract temporal features.
\item \textbf{GWN}\cite{wu2019graph}: This approach incorporates a learnable graph structure to model spatial correlations, while TCNs are used to extract temporal features.
% \item \textbf{STSGCN}~\cite{Song2020spatial}: This model synchronously models dynamic ST correlations by constructing a graph network that allows interactions across time slices.
\item \textbf{STSGCN}\cite{Song2020spatial}: It synchronously models dynamic spatio-temporal correlations by constructing a graph network that allows interactions across time slices.
% \item \textbf{MTGNN}~\cite{wu2020connecting}: This method captures temporal dependencies using time convolutional networks combined with skip connections, and employs learnable graph networks to model spatial correlations.
\item \textbf{MTGNN}\cite{wu2020connecting}: This method captures temporal dependencies using time convolutional networks combined with skip connections, and employs learnable graph networks to model spatial correlations.
% \item \textbf{STFGNN}~\cite{li2021spatial}: In this method, a data-driven spatio-temporal graph construction approach is proposed to capture dynamic spatio-temporal correlations.
\item \textbf{STFGNN}\cite{li2021spatial}: This method proposes a data-driven spatio-temporal graph construction approach to capture dynamic spatio-temporal correlations.
% \item \textbf{DMSTGCN}~\cite{han2021dynamic}: This method models dynamic spatial correlations by constructing a learnable dynamic graph network.
\item \textbf{DMSTGCN}~\cite{han2021dynamic}: This method models dynamic spatial correlations by constructing a learnable dynamic graph network.
\end{itemize}

\noindent \textbf{Attention-based Spatio-Temporal Models:}
\begin{itemize}[leftmargin=*]
% \item \textbf{ASTGCN}~\cite{Guo2019attention}: This method utilizes attention mechanisms for periodic modeling of ST correlations.
\item \textbf{ASTGCN}\cite{Guo2019attention}: This method leverages attention mechanisms to model periodic spatio-temporal correlations.
% \item \textbf{STWA}~\cite{cirstea2022towards}: This approach injects specialized node features and time dynamic parameters into attention mechanisms to jointly model dynamic spatio-temporal correlations.
\item \textbf{STWA}\cite{cirstea2022towards}: This approach incorporates specialized node features and time dynamic parameters into attention mechanisms to jointly model dynamic spatio-temporal correlations.
% \item \textbf{PDFormer}~\cite{jiang2023pdformer}: This model encodes spatio-temporal dependencies based on the transformer architecture. Additionally, a time-delayed spatial correlation modeling is designed to more accurately simulate real-world traffic scenarios.
\item \textbf{PDFormer}~\cite{jiang2023pdformer}: This model encodes spatio-temporal dependencies using the transformer architecture. Additionally, it introduces a time-delayed spatial correlation modeling technique to more accurately simulate real-world traffic scenarios.
\end{itemize}

\textbf{ODE-based Spatio-Temporal Prediction Method:}
\begin{itemize}[leftmargin=*]
% \item \textbf{STGODE}~\cite{fang2021spatial}: This method enhances graph networks with ordinary differential equations (ODEs) to extract continuous spatial correlation information. Time convolutional networks are used to learn time-dependent relationships.
\item \textbf{STGODE}~\cite{fang2021spatial}: This method enriches graph networks with ordinary differential equations (ODEs) to extract continuous spatial correlation information. Time convolutional networks are employed to learn time-dependent relationships.
\end{itemize}

% \begin{table}[htbp]
%     \centering
%     \vspace{-0.1in}
%     \caption{Statistics of pre-training dataset.}
%     \label{tab:Dataset_pretrain}
%     \scalebox{0.69}{
%     \begin{tabular}{c|c|c|c|c}
%         \hline
%         Dataset & Data Record & \# Region & Time Steps & Sample Date\\
%         \hline
%         PEMS03 & traffic flow & 358 & 26208 & 1/Sep/2018 - 30/Nov/2018 \\
%         PEMS04 & traffic flow & 307 & 16992 & 1/Jan/2018 - 28/Feb/2018\\
%         PEMS07 & traffic flow & 883 & 26208 & 1/May/2017 - 30/Aug/2017\\
%         PEMS08 & traffic flow & 170 & 17856 & 1/Jul/2016 - 31/Aug/2016\\
%         \hline
%     \end{tabular}
%     }
%     % \vspace{-0.15in}
% \end{table}

% \begin{table}[htbp]
%     \centering
%     \vspace{-0.1in}
%     \caption{Statistics of downstream tasks dataset.}
%     \label{tab:Dataset_test}
%     \scalebox{0.65}{
%     \begin{tabular}{c|c|c|c|c}
%         \hline
%         Dataset & Data Record & \# Region & Time Steps & Sample Date\\
%         \hline
%         PEMS07(M) & traffic speed & 170 & 12672 & 1/Jul/2016 - 31/Aug/2016\\
%         CA-D5 & traffic flow & 211 & 16992 & 1/Jan/2017 - 28/Feb/2017 \\
%         ChengDu-DIDI & traffic index & 524 & 17280 & 1/Jan/2018 - 30/Apr/2018\\
%         NYC Citi Bike & bike orders & 250 & 4368 & 1/Apr/2016 - 30/Jun/2016\\
%         \hline
%     \end{tabular}
%     }
%     % \vspace{-0.15in}
% \end{table}

\textcolor{red}{\textbf{Complexity Analysis of the \model\ Framework.} In terms of computational complexity, the temporal dependency encoder in the spatio-temporal dependency modeling component has a complexity of $O(L\times F \times R \times d'^2)$, while the spatial dependency encoder has a complexity of $O(L \times F \times R \times d'^2 + L \times F \times E \times d')$. Here, $L$ represents the number of layers in the spatio-temporal encoder, and $E$ denotes the number of edges. The spatio-temporal context distillation utilizes simple linear layers, resulting in a lower complexity compared to the spatio-temporal dependency modeling. The infoNCE loss function $L_{Uni}$ employed for adjusting the embedding distribution in the unified distribution mapping mechanism has a complexity of $O(F \times R^2 \times d')$. Overall, the \model\ framework exhibits lower computational complexity compared to other spatio-temporal baseline models. This characteristic enables our proposed method to efficiently adapt to downstream tasks.}

\textcolor{red}{\textbf{Limitations of the Proposed Framework.} In this work, we introduced the \model, which has been validated to effectively enhance the generalization capabilities of downstream models across various spatio-temporal data scenarios. However, there are some limitations to this work. Given the broad scope of spatiotemporal prediction tasks, the proposed method may not be suitable for all spatio-temporal tasks. For instance, while \model\ is pre-trained on traffic flow datasets, it might underperform in downstream tasks such as weather forecasting, due to the substantial difference in the knowledge that needs to be learned (e.g., a weather forecasting model may not benefit from understanding traffic patterns during rush hours). Therefore, when applying \model\ to new spatio-temporal tasks, we recommend first assessing the relevance between the pre-training and the downstream tasks. Pre-training on data from related tasks can yield better performance evaluations.}
